# Supplementary material for: SplatFormer: Point Transformer for Robust 3D Gaussian Splatting
Source: arXiv:2411.06390 source file (2025-03-10)
Supplement: Supplementary file 1 [file supp_results-objaverse.bkup.tex]

\begin{figure}[t!]
    % \vspace{-1em}
    \centering
    \scriptsize % Sets the text within the figure to a smaller font size.
    \setlength{\tabcolsep}{0mm} %0 Adjusts the spacing between columns in the table. A small value creates tightly packed columns.
    \newcommand{\sz}{0.120}  % 0.33 Defines a new command \sz to represent a size fraction (16% of the linewidth). This size is used later to control image sizes.
     %Reduces the vertical space between rows in the table to near zero, making rows more compact.
    % Define a new command that compares one example across multiple methods
    \newcommand{\compareexamplerow}[1]{
            \begin{tabular}{ccccccc}
            Four of Inputs&\text{MipNeRF360}&\text{Nerfbusters}&\text{InstantNGP}&\text{SyncDreamer}&\text{LaRa}&\text{SSDNeRF} \\
            \includegraphics[width=\sz\linewidth]{Figures/results/#1_gt_2x2} &\hspace{1mm}
            \includegraphics[width=\sz\linewidth]{Figures/results/#1_mipnerf360} &
            \includegraphics[width=\sz\linewidth]{Figures/results/#1_nerfbusters} &
            \includegraphics[width=\sz\linewidth]{Figures/results/#1_instantngp} &
            \includegraphics[width=\sz\linewidth]{Figures/results/#1_syncdreamer} &
            \includegraphics[width=\sz\linewidth]{Figures/results/#1_lara} &
            \includegraphics[width=\sz\linewidth]{Figures/results/#1_ssdnerf} \\
            % \vspace{3mm}
% \phantom{+++}&\phantom{+++}&\phantom{+++}&\phantom{+++}&\phantom{+++}&\phantom{+++}&\phantom{+++}\\
\text{GT}& \text{Ours}&\text{2DGS}&\text{SplatFields}&\text{FSGS}&\text{3DGS}& \text{InstantSplat} \\
            \includegraphics[width=\sz\linewidth]{Figures/results/#1_gt} &\hspace{1mm}
            \includegraphics[width=\sz\linewidth]{Figures/results/#1_ours} &
            \includegraphics[width=\sz\linewidth]{Figures/results/#1_2dgs} &
            \includegraphics[width=\sz\linewidth]{Figures/results/#1_splatfield} &
            \includegraphics[width=\sz\linewidth]{Figures/results/#1_fsgs} &
            \includegraphics[width=\sz\linewidth]{Figures/results/#1_3dgs} &
            \includegraphics[width=\sz\linewidth]{Figures/results/#1_instantsplat} \\
\phantom{+++}&\phantom{+++}&\phantom{+++}&\phantom{+++}&\phantom{+++}&\phantom{+++}&\phantom{+++}\\
\phantom{+++}&\phantom{+++}&\phantom{+++}&\phantom{+++}&\phantom{+++}&\phantom{+++}&\phantom{+++}\\
            \end{tabular}
    } %Define a new command to include images with common formatting
\compareexamplerow{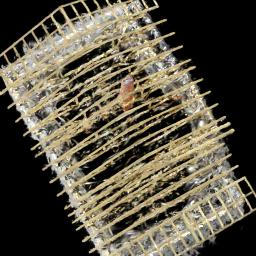}
\compareexamplerow{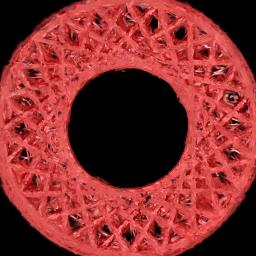}
% \compareexamplerow{914d43018c9b4cd681e31d56cb889563-10-test_elevation90_step1} red car
% \compareexamplerow{3e66059c275548c4a183b2f9e085f953-10-test_elevation90_step2} %plane as failure case
\compareexamplerow{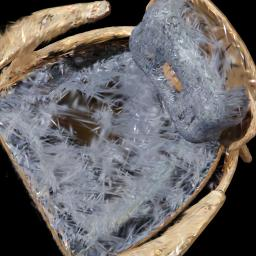}
\compareexamplerow{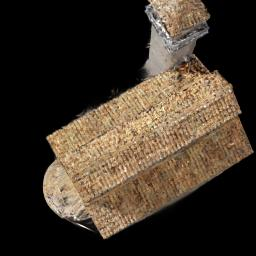}
% \compareexamplerow{0af0dfc6afd045d9990aa688f6c792ff-20-test_elevation70_step1}
% \compareexamplerow{0a6e1a80d2e34d5981d6b2b440bbc8cd-10-test_elevation90_step1} blue jet
\compareexamplerow{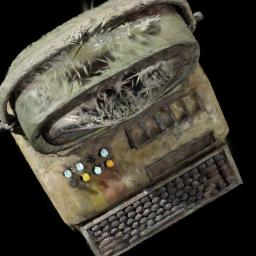}
% \compareexamplerow{5fcd426a7d754a95b64ea21f34b762ea-10-test_elevation80_step2}
% \compareexamplerow{81fe61e043ba411c951e4b3b80e82ca4-20-test_elevation80_step2}

% \compareexamplerow{3a64ef3f2e8a4b4f9d3ebdb835053df9-20-test_elevation90_step2}

    \caption{\textbf{Results on Objaverse-OOD.} We compare our method with baselines: SyncDreamer~\citep{liu2023syncdreamer}, LaRa~\citep{LaRa}, SSDNeRF~\citep{ssdnerf}, 3DGS~\citep{kerbl3dgs}, Nerfbusters~\citep{Nerfbusters2023}, SplatFields~\citep{SplatFields}, InstantSplat~\cite{fan2024instantsplat}, 2DGS~\citep{huang20242dSplat_Tuebingen}, FSGS~\citep{zhu2023FSGS_texas}, InstantNGP~\citep{mueller2022instantngp}, and MipNeRF360~\citep{barron2022mipnerf360}.} 
    \label{fig:exp_full_objaverse}
\end{figure}

% %In main text:
% \input{figures_tex/exp_static_recon}
