# Supplementary material for: SplatFormer: Point Transformer for Robust 3D Gaussian Splatting
Source: arXiv:2411.06390 source file (2025-03-10)
Supplement: Supplementary file 2 [file supp_efficiency.tex]

\begin{wraptable}[7]{r}{7.0cm} % [19]
    \scriptsize
    \setlength{\tabcolsep}{0.6pt}
    \vspace{-2em}
    \caption{\textbf{Memory Usage and Inference Time.}} \label{tab:supp_efficiency}
 \resizebox{7.0cm}{!}{
    \begin{tabular}[t]{c|ccc|c}
    \toprule
      Number of Splats & 10k–40k & 60k–70k & 90k-100k & Average \\
    \midrule
      Memory (MB)&675&801&1010&782\\
      Time (ms)&62&70&118&75\\
    \bottomrule
    \end{tabular}
}
\end{wraptable}
